# Supplementary material for: High-Resolution Swin Transformer for Automatic Medical Image Segmentation
Source: arXiv:2207.11553 source file (2022-07-23)
Supplement: Supplementary file 1 [file sec_supplementary.tex]

\section{Supplementary Material}
